# Supplementary material for: Extracting Shopping Interest-Related Product Types from the Web
Source: arXiv:2305.14549 source file (2023-05-23)
Supplement: Supplementary file 1 [file a5-feedback.tex]

\section{Feedbacks}

\subsection{Abstract}

L9: "extracting the shopping interest-related product types from the internet" comes as a suprise. Why this problem?
\yliinline{Addressed.}

L15: "Instead of several selected websites" seems to implicitly indicate we are targeting the Web. We need to draw the reader gradually into our approach. For example, something like "While the PT mining problem can be approached via manual curation and/or connecting an interest directly to products, the former can be limited in their scalability to a large set of interests or can be ineffective since products seldom indicate the wide range of applications where they can be used, e.g. Cooler product may not mention its use toward graduation party."
\yliinline{Partly addressed. Provided simpler explenations instead. I'm putting the detail in Intro to reduce Abs length.}

L21: "as a binary node classification task". I think we should briefly say that this is different from existing extraction problem, which is why we require a new model.
\yliinline{Addressed.}

L36: Let's state the best performance here.
\yliinline{Addressed.}

\subsection{Introduction}

L45-L63: I think this needs more details and refinement. 
\begin{itemize}
	\item I think we can talk about lower and upper-funnel customer segments (since these notions are well-studied in marketing) and that we are interested in helping the customers in the upper shopping funnel category. Example: https://www.convertcart.com/blog/ecommerce-conversion-funnel
	\item We should talk about what people do today. We should use an interest as a running example throughout the paper. Fofjcbfdjvecr example, today, a customer interested in knowing essential items during a COVID-19 outbreak ("COVID-19 crisis") is only shown a listing of books on the topic. Therefore, people often perform their product research on the Web, relying on hand-curated websites (e.g., rei.com for camping), before coming to an ecommerce website to purchase their products. This way, the customers have become accustomed to using the ecommerce website only when they have determined specific products or the kind of products they want. 
	\item We should then talk about the end experience we want to deliver: we aim to help the upper-funnel customers by helping them research and discover products directly on the ecommerce platform, making it a one-stop shop for all their interest-oriented needs. Such discovery experience can be delivered via product recommendations and/or search. Example of an envisioned search system is shown in Figure 1, where the system shows an organization of products categorized by product types relevant to a given interest.
\end{itemize}
\yliinline{addressed}

L65: Before talking about automatic data mining, we should briefly discuss what naive or simple approaches can one explore to connect an interest to relevant products: curation, search of interests in product description, establishing semantic association between interest and product via their latent space embeddings, etc., followed by where each of them falls short.

L67: We need a figure showing representative webpage containing a list of surface PTs. The readers may not have clue what kind of websites we are referring to. Here we should also talk about any observations regarding these websites, e.g. are these templated? "hub pages"? what kinds of data typically exists on a page? what characteristics are common across sites (presence of bullet points)? what is different from site to site?

L76: State the problem first: we are interested in finding surface-level product types (e.g. "camping tent") in a given webpage that are relevant to an interest and mapping them to well-defined product types in an existing product taxonomy. Given an example, for an interest such as "camping", we hope to discover camping tent, sleeping bag, inspect repellent, first-aid kit, flashlight, etc. as relevant product types.

L85: "[The problem] is non-trivial .." talking about challenges can benefit from having an enumerated list of key challenges.
\begin{itemize}
	\item Website heterogeneity: Each website displays content in a different format and terminology, so a solution designed for one or few websites may not work for others.
	\item Noise vs. relevant PTs: Webpages often contain listing of product types interspersed with long descriptive text and images (correct me in case wrong)
	\item Generalization to unseen interests: Identifying PTs relevant to any given interest is a fundamental challenge. Tailoring our extraction approach for a few interests seen during training may not allow generalization to other interests, thereby demanding us to consider a zero-shot setup.
\end{itemize}

L108: I think we should briefly contrast this problem with attribute extraction work and point out why none of its approaches are applicable here.

L126: Start with the main extraction challenge and give a brief high-level intuition behind the proposed model's use of ancestor-descendant and sibling relations.

L145: 3% gain "per F1 score". Also what is the best performance on this dataset?

L150: Omit words like "influential". Consider rephrasing to something like "We consider a novel problem of product type extraction from the Web for a given set of shopping interests".

L155: "We provide a manually constructed dataset.." -> Do we want to be explicit? Amazon Legal will certainly probe on this. "We make our manually curated dataset publicly available to promote more research on this problem."

\subsection{Problem Setup}

L233: "arbitrary website" - Don't we mean relevant websites identified by the website selection phase?

\subsection{Method}

L244: Have a short overview of the solution before delving into input features and Treeformer architecture details. Start with the key intuition and how we aim to model the problem using available signals (HTML structural information, DOM node text sequences, shopping interests). The idea would be to first give a high-level picture of the solution (consider having a figure), followed by details of each "building block". 

I will provide comments on individual subsections later.

\subsection{Experiment}

L449: "There is no previous work.. for tree node classification". Many of the attribute extraction approaches do node classification, so sounds like this statement needs more context.

L493: SIPT-INT-i means i'th partition of interests in the Shopping-interest PT Extraction dataset? Let's have a simpler naming scheme; may cause confusion unnecessarily; it did for me :) Also, this makes me think we should name our dataset if we plan to make it publicly accessible.

L535: Table 1: Would help to order the rows by increasing average F1. 

Will read up details and give more specific details on Experiment and Conclusion later this week.
